# Supplementary material for: Understand Data Preprocessing for Effective End-to-End Training of Deep Neural Networks
Source: arXiv:2304.08925 source file (2023-04-18)
Supplement: Supplementary file 1 [file appendix.tex]

\section{Appendix-Summary}
\label{sec:appendix}

\subsection{Meeting note for Feb 18, 2020}

\subsubsection{Main discussion points}
\begin{itemize}
    \item Overview of DNN training process including the data consuming patterns
    \item Overview of the data loading pipeline for the three popular dnn frameworks such as Tensorflow, Pytorch and MXnet
    \item Summary of the similarities, differences and potential problems of these data loading pipelines
\end{itemize}

\subsubsection{Comments from audience}
\cheng{@Ping and @Yuxin, please complete this part.}
\begin{itemize}
    \item From Sam: Focusing on one framework and CNN, try to find the evidences about the problem of data loading. 
    \item From Xiaosong: Comparison across framework might be interesting. Figure out which part we should work for, data organization or overlap between reading and processing or others.
    \item From both: If the problem exists, please figure out the fundamental issues that trigger these problems.
\end{itemize}

\subsubsection{Next steps}
We will focus on evaluating the impacts of enabling data loading pipeline on the overall training process with default settings. Here, we only target \textbf{Tensorflow} and \textbf{Pytorch}, and we distribute the workload among Ping and Yuxin evenly, where Ping is responsible for testing Tensorflow, while Yuxin will be working with Pytorch. Then, we identify potential performance issues. Finally, we have to compare the performance numbers between Tensorflow and Pytorch.

Next, please write the following information in the evaluation section~\ref{sec:eval:explore}.

\begin{itemize}
    \item Please first find the DNN model we want to evaluate. The training process of this model should be fast, and the batch size should be large, so that we can clearly see the stress on data loading.
    \item Please also think about which set of parameters we should set for the whole data loading pipeline. Please include a table in the text to describe those parameters, e.g., meaning, belong to which stages of the pipeline, impacts, range, etc.
    \item Please also tell us what are the metrics that you want to evaluate and which set of figures you want to draw.
\end{itemize}
